# Supplementary material for: Stability and Scalability of Blockchain Systems
Source: arXiv:2002.02567 source file (2020-12-19)
Supplement: Supplementary file 1 [file rebuttal-appendix.tex]

\newpage
\section{Response to the Reviewer Comments}
In this section we address the reviewers' comments from our earlier submission.
We thank the reviewers for their insightful comments and feedback which have helped us improve the depth and presentation of our results.
Below, we address the reviewers's specific comments.


First, we address the shepherd's concerns with each concern highlighted in bold and our response following. 
Subsequently, we respond to concerns raised by the individual reviewers.

\subsection{Response to Shepherd}

\begin{enumerate}
    \item {\bf Clarify the meaning and significance of $G(\infty)$ and ``one-endedness"}. \\
    The DAG $G(\infty):=\cup_{t \geq 0} G(t)$ is defined as the union of blockchain DAGs at all time $t \geq 0$. 
    This corrects an important typographic error from the last submission.  
    % We have added a new section, Section \ref{sec:structural-properties}, which discusses the importance of a one-ended limit in a blockchain system in terms of having an increasing number of 
    The relevance of one-endedness has been added in Section \ref{sec:one-ended-infinite_confirm}, which shows that if $G(\infty)$ is one-ended, then there will be infinitely many confirmed blocks (Definition \ref{def:confirmed}). 
    The importance of having a one-ended limit is also discussed in Section \ref{sec:one_end_dist_consensus}, where having infinitely many confirmed blocks is a structural way of describing distributed trust.
    
    Please also refer to the discussions on ``Infinite DAGs and Asymptotic Properties'' and ``One-Endedness and Blockchain Systems'' below for more explanation and details.
    
    \item {\bf What are the Markovian assumptions that the authors consider to be able to produce a Markov model amenable to analysis in the limit? Discuss whether these assumptions are reasonable.}
    \\
    
    
    In the theoretical analysis, the only distributional assumption we use is that the peers communicate among each other at epochs of a Poisson Process.
    We use this model, guided by the measurement study in \cite{decker2013information} which observes that the information propagation resembles a Markovian gossip process.
    We do not make any assumption on the block arrival process, except that it is stationary and ergodic.
    In this sense, our model is not Markovian, as a Markovian blockchain model would require both Poisson transmission processes as well as Poisson arrivals.
    
    Please refer to the discussion on ``Validity of Markovian Assumptions" below for a detailed discussion.
    
    
    \item {\bf Clarify characteristics of the metrics and properties that the paper seeks to investigate} \\
    The key property studied in this paper is to characterize when a blockchain system is stable and scalable. 
    Furthermore, when the system is stable, we present more fine-grained metrics in Section \ref{sec:interpretations} and \ref{sec:simulations}, which allows us to further understand and characterize the P2P network behavior.
    
    Refer also to the following discussion on ``Stability and Scalability.''
    
    \item {\bf Make precise all the metrics associated with the infinite graph $G(\infty)$ that are relevant to this work, and which of them have a limiting behavior}.\\
    The main property of the infinite limiting DAG $G(\infty)$ that we consider is that of ``one-endedness" (defined in Definition \ref{def:one-ended}). 
    See also the discussion on ``Infinite DAGs and Asymptotic Properties" in the sequel.
    
    \item {\bf Explain the difference between "stability" and "scalability"}.
    \\
    The goal of a blockchain system is to achieve consensus by confirming blocks.
    Stability implies that there is a positive rate at which blocks can be confirmed on a fixed P2P network.
    Scalability implies that there is a fixed positive rate for which a sequence of P2P networks with increasing numbers of peers are all stable.
    
    Please also refer to the discussion under ``Stability and Scalability."
    
    \item {\bf  Section 3.1: "Properties and Definitions" defines the concept of "consistent". Strangely, none of the lemmas/ theorems/propositions involve any discussions on "consistency". Make explicit use of the the concept of "consistency" and of that term throughout the paper}.\\
    
    The definitions of stability and scalability rely on the notion of consistency (see Definition \ref{def:stability} and \ref{def:scalability}). 
    In this sense, the definition of consistency is explicitly used throughout the paper.
    
    \item {\bf Indicate the applicability of the model. For that purpose, the best is to present real world data about \\
    blockchains to support the work.}
    \\
    We conducted experiments with real data traces in addition to the synthetic experiments presented in the previous submission. 
    The new experiments consist of both more detailed simulations (using realistic system parameters obtained from literature) and simulations using data collected from the Bitcoin blockchain (for block inter-arrival times).
    We refer to the discussion under the heading ``Real Data Traces.''
    
    \item {\bf Clearly relate the work to all prior art on classic and recent advances in p2p stability as well as queueing models for blockchain systems.}
    \\
    We thank the reviewers for the detailed list of references; many of these are now included in the Related Work in Section \ref{sec:related_work}.
    
    See also the following discussion on ``Connections with Prior Work'' in the sequel.
\end{enumerate}


\subsection{Detailed Response to Reviewers}

\noindent{\textbf{Connections with Prior Work}} --
We remark that although our model looks similar to those studied in the peer-to-peer and gossip algorithms literature and the queueing literature, it qualitatively differs from the canonical setup in either of them.
The P2P gossip literature assumes that the set of information to be disseminated is not generated as time progresses, but is assumed to be fixed beforehand.
In contrast, in our model, the information to be disseminated is the set of blocks, which arrive over time.
Similarly, our model resembles a queueing system, where blocks represent customers, and a block is in ``service'' in a generalized processor sharing queue as long as there exists at least one peer missing it, and the block departs the queue when all peers are aware of this block.
However, the state of the process cannot just be captured by queue length, as the services of different blocks (customers) in the queue are dependent on the underlying gossip process.

\noindent {\bf Comparison of Stability Criterion with \cite{papadis2018stochastic}} -- A significant difference between our model and that of \cite{papadis2018stochastic} is the fact that the `service rate' of a block is not fixed or hard-coded in our model. 
Rather, a block is in `service' in the network as long as not all peers are aware of the block. 
Thus, the rate at which blocks `leave the system' depends on the instantaneous state of network congestion.
In this sense, there is no `obvious' guess or conjecture for the stability criterion as in the model in \cite{papadis2018stochastic}.
In particular, blocks in the Bitcoin network arrive at a desired rate of $1$ block per $600$ seconds.
This is the the block arrival rate; the validation rate depends on the gossip process and network congestion.

\noindent{\textbf{Infinite DAGs and Asymptotic Properties}} -- 
In order to increase readability,
we include a subsection (Section \ref{sec:definitions}) to clearly highlight the non-standard graph theoretic definitions we use in this work.
This was suggested by Reviewer A and we believe that it significantly improves the structure of our paper.

We also thank the reviewers for pointing out an important typographic error in the initial draft, that ``$G(\infty) := G(t)$.'' 
It should read, ``$G(\infty) := \cup_{t\geq0}G(t)$,'' and this change is reflected in the paper.
Thus, the (random) DAG $G(\infty)$ is the union of the random blockchain DAGs $G(t)$ for all times $t \geq 0$.
It is in this sense that we speak of of $G(\infty)$ as a limit of the DAG $G(t)$.
Moreover, $G(\infty)$ is a limiting random DAG and is not an evolving DAG with time.
Moreover, as we define $G(\infty)$ as a union, its existence is trivial.

Further work involving limits of (growing) finite graphs and infinite evolving graphs can be found in several sub-fields of engineering and applied mathematics, such as in social networks (\cite{acemoglu2011bayesian}), mathematical physics (\cite{sander1986fractal, eden1961two, mihail2003certain}), and unimodular random graph theory (\cite{aldous2007processes, baccelli2018renewal, baccelli2018eternal}).
Motivated by this, in our work we examine asymptotic blockchain properties by taking the limit of finite DAGs as the number of vertices grows; Acemoglu \textit{et al.} \cite{acemoglu2011bayesian} take a similar limit to study opinion dynamics in social networks.
Growth processes, in which graphs are grown sequentially, have long been studied in mathematical physics and have been used to model fractals \cite{sander1986fractal, eden1961two}.
In addition, the commonly used preferential attachment model of the connectivity of the internet structure \cite{mihail2003certain}, is also a growth process.
See \cite{aldous2007processes, baccelli2018renewal, baccelli2018eternal} for studies of infinite evolving graphs and unimodularity, which is a form of stationarity for infinite rooted graphs.

\noindent{\textbf{One-Endedness and Blockchain Systems}} -- As a result of reviewer feedback, we have changed our presentation of the concept of one-endedness and its significance in the analysis of blockchain systems.
We have added a new section (Section \ref{sec:structural-properties} in this revised version), which argues that it is desirable for the blockchain system to be such that the limiting DAG $G(\infty)$ be one-ended. 
More precisely, we show in Lemma \ref{lem:one-ended-confirmed}, that if $G(\infty)$ is one-ended and localy finite, then there exists 
infinitely many confirmed blocks (see Definition \ref{def:confirmed}).
 The confirmed blocks are the ones that all peers trust (see Propositon \ref{prop:trust}); thus since infinitely many blocks arrive to the system, it is desirable to also have infinitely many of those blocks confirmed.
Our main result in this paper (Theorems \ref{thm:tree-one-ended} and \ref{thm:throughput-optimal-one-ended}) is to prove that if the blockchain system is stable, then  the limiting blockchain DAG $G(\infty)$ is one-ended, which in turn from Lemma \ref{lem:one-ended-confirmed} provides a sufficient condition on the blockchain system parameters for infinitely many blocks to be confirmed.

% Our result in Lemma \ref{lem:one-ended-confirmed} provides a sufficient condition, whereby if the limiting graph $G(\infty)$ is one-ended, then there will be infinitely many confirmed blocks. 

% More precisely, we show in Lemma \ref{lem:infinitely-confirmed}, that if the limiting graph $G(\infty)$ is locally finite and contains infinitely many confirmed blocks (see Definition \ref{def:confirmed}), then the subgraph of $G(\infty)$ consisting only of the confirmed blocks is one-ended.
% Further, we show (Lemma \ref{lem:one-ended-confirmed}) that the one-endedness and local finiteness of $G(\infty)$ together imply the existence of infinitely many confirmed blocks.
% As we argue in the paper in Section \ref{sec:structural-properties}, a desirable property of blockchain systems is to have infinitely many confirmed blocks in the limit as time $t \to \infty$. 
% The confirmed blocks are the ones that all peers trust (see Propositon \ref{prop:trust}); thus since infinitely many blocks arrive to the system, it is desirable to also have infinitely many of those blocks confirmed.
% Our result in Lemma \ref{lem:one-ended-confirmed} provides a sufficient condition, whereby if the limiting graph $G(\infty)$ is one-ended, then there will be infinitely many confirmed blocks. 
% Our main result in this paper (Theorems \ref{thm:tree-one-ended} and \ref{thm:throughput-optimal-one-ended}) is to prove that if the blockchain system is stable, then  the limiting blockchain DAG $G(\infty)$ is one-ended. 

\noindent{\textbf{Stability and Scalability}} -- 
Our reviewer feedback noted that we did not provide precise definitions for stability or scalability.
While these are commonly used terms in the literature involving stochastic networks, we have added definitions to the paper in Section \ref{sec:stability-scalability} for increased readability to a wider audience.
Roughly speaking, we say the blockchain system is stable if there exists a positive arrival rate such that infinitely many blocks are confirmed (for a fixed P2P network).
Scalability, on the other hand, assesses, whether there exists a positive arrival rate that is stable for a sequence of P2P networks that grow in size, \textit{i.e.}, scalability is an asymptotic property as space (P2P network size) goes to infinity.

We have added a new section on the scalability of blockchain systems (Section \ref{sec:scalability}).
In that section, we analyze the scalability of P2P networks of various common network topologies.
A key result in this paper (Theorem \ref{thm:stability}) provides a sufficient condition to determine when a sequence of P2P networks is not scalable (see discussions in Section \ref{sec:scalability}).

% In particular, in the Introduction, we note that a significant challenge to the blockchain system community is that of throughput optimization; we discuss how throughput optimization depends on stability and scalability to highlight the importance of our analysis and any future analyses.

In addition, it was noted that we do not use the term consistency, even though it is defined.
The definitions of stability and scalability depend on consistency (Definition \ref{def:consistent}), and the wording of Theorems \ref{thm:tree-one-ended} and \ref{thm:throughput-optimal-one-ended} (and their associated Lemmas) have been edited to reflect the terminology of consistency and stability.

\noindent{\textbf{Validity of Markovian Assumptions}} -- 
Our previous submission used the assumption of Markovian dynamics to do the theoretical stability analysis in Section \ref{sec:stability} -- namely we assumed that all transmissions and arrivals are mutually independent Poisson processes.
In this revision, we relax this Markovian assumption, and treat the block arrival process as a general stationary and ergodic process.
However, we keep the gossip communication process among peers as a Poisson Point Process, which is the only Markovian assumption made in this paper.
This assumption of Poisson gossip-based communications among peers is consistent with the implementation of the Bitcoin blockchain \cite{nakamoto2008bitcoin, fanti2018dandelion++}.
% In our simulated characterization of our metrics in Section \ref{sec:simulations}, we set the arrival process as a Poisson process for simplicity.

We remark that there have been several measurement studies of the Bitcoin network that validate these assumptions.
Specifically, Decker and Wattenhofer \cite{decker2013information} find that information propagation in blockchain systems resembles gossip-based P2P information dissemination.
This observation motivates our communication model among peers
which occurs at epochs of a Poisson process.
A typical assumption made in the blockchain lterature (for example, see \cite{nakamoto2008bitcoin, bagaria2019prism, papadis2018stochastic}) is that the block arrival process is Poisson.
In this paper however, we present the theoretical results without assuming Poisson block arrivals.
Furthermore, using real data traces for block arrival times (see the discussion on ``Real Data Traces'' in the sequel), we also verify the validity of modeling block arrivals as a Poisson process.


% The Poisson arrival assumption of  is widely made in the literature (\cite{nakamoto2008bitcoin, bagaria2019prism, papadis2018stochastic}.
% Our experimental results (see Tables \ref{tab:time_to_consistency}, \ref{tab:cycle_length}, \ref{tab:consistency_fraction},\ref{tab:age_of_information}) with real data traces validates this modelling assumption.



%and experimental setup, in which we compare metrics for our model with Poisson inputs and real data traces for block arrival times.


\noindent{\textbf{Real Data Traces}} -- 
Our experimental study in Section \ref{sec:simulations} consists of two setups, a synthetic setup (similar to the previous submission) and a new setup with real data traces of the Bitcoin network.

% %Inspired by the reviewers' comments from the last submission, we conduct in Section \ref{sec:simulations}, a study using real data trace of the Bitcoin blockchain.
In the real data experimental setup, we use real data traces from \cite{blockchair2020data}, which gives the arrival times of blocks into the system.
This data set consists of 2000 blocks generated between dates December 27, 2019 and January 09, 2020.
We then use this data set to specify arrival times of blocks into a network of peers.
To model the P2P network, we use measurements from 
\cite{decker2013information} and \cite{gencer2018decentralization}, which give approximate values for the number of peers, average degree, and average bandwidth in the Bitcoin network.
With this experimental setup, we analyze the network performance and report various metrics in Section \ref{sec:simulations}.
We find, through our experimental results, that the observed performance metrics are close to what would have been observed if the blocks arrived into the system as a Poisson process as opposed to using the real data traces.

In the synthetic experiments, we assume that the block arrivals follow a Poisson process, and the network among the agents is the complete graph. 
This experimental setup allows us to assess the impact of block arrival rate on performance metrics (identified in Section \ref{sec:interpretations}).
This is only possible with synthetic data, as the real data set consists of a single arrival process of blocks and thereby we cannot use it directly to assess the impact of varying the block arrival rate on performance.
